# Supplementary material for: Did They Really Tweet That? Querying Fact-Checking Sites and Politwoops to Determine Tweet Misattribution
Source: arXiv:2211.09681 source file (2022-11-17)
Supplement: Supplementary file 1 [file Appendix.tex]

\begin{center}
\bf{Figures, Tables and Other templates}
\end{center}

Lists are easy to create: Use "[noitemsep,topsep=0pt]" to remove space between each entries.
\begin{itemize}[noitemsep,topsep=0pt]
  \item List entries start with the \verb|\item| command.
  \item Individual entries are indicated with a black dot, a so-called bullet.
  \item The text in the entries may be of any length.\\
\end{itemize}

Numbered (ordered) lists are easy to create. Here's a list with spacing
\begin{enumerate}
  \item Items are numbered automatically.
  \item The numbers start at 1 with each use of the \texttt{enumerate} environment.
  \item Another entry in the list
\end{enumerate}

\begin{figure}[h!]
  \centering
  \includegraphics[width=0.40\linewidth]{figs/op.png}
    \vspace*{-4mm}
  \caption{Human Oculomotor Plant}
  \label{fig:op}
\end{figure}

%%%%%%%%%%%%%%%%%%%%%%%%%%%%%%%%%%%%%%%%%%%%%%%%%%%%%%%%%%%%

\begin{figure}[h!]
  \centering
  \includegraphics[width=0.60\linewidth]{figs/OPF.jpg}
    \vspace*{-4mm}
  \caption{Oculomotor Plant Feature Estimation Process \cite{jayarathna2016rationale}}
  \label{fig:opf}
\end{figure}

%%%%%%%%%%%%%%%%%%%%%%%%%%%%%%%%%%%%%%%%%%%%%%%%%%%%%%%%%%%%

\begin{figure*}[t]
\centering
\fbox{
\includegraphics[width=.46\linewidth]{figs/subflow-datamux-in.png}
}
\fbox{
\includegraphics[width=.46\linewidth]{figs/subflow-datamux-out.png}
}
\caption{
\textbf{Multiple images examples.}
\textnormal{The \textit{Images} (left) Left image (right) Right image.}
\label{fig:subflow}
}
\end{figure*}

%%%%%%%%%%%%%%%%%%%%%%%%%%%%%%%%%%%%%%%%%%%%%%%%%%%%%%%%%%%%

\begin{table}[h!]
    \centering\scriptsize
   \caption{\footnotesize Faculty participants of this REU Site proposal. IR: Information Retrieval; HCI: Human Computer Interaction; NLP: Natural Language Processing; ML: Machine Learning; DL: Digital Libraries; WS: Web Science. \label{tab:faculties}}
    \begin{tabular}{c|c|c|c|p{6.5cm}}
    \toprule
    {\bf Role} & {\bf Name}     &  {\bf Title} & {\bf Affl.} & \multicolumn{1}{c}{\bf Expertise}\\
    \midrule
    PI \& Mentor & Sampath Jayarathna & Asst. Prof.& CS & Data Science, Eye tracking, HCI, IR, ML\\ \midrule
    Co-PI \& Mentor     & Jian Wu & Asst. Prof. & CS & NLP, Scholarly Big Data, IR, Data Mining\\ \midrule
    Mentor & Michael Nelson & Prof. & CS/VMASC & DL, Web Archiving, WS, Data Science, Social Media\\ \midrule
    Mentor & Michele Weigle & Prof.&CS & WS, Data Visualization, Social Media\\ \midrule
    Mentor & Vikas G. Ashok & Asst. Prof.&CS & Accessible Computing, HCI, NLP\\ \midrule
    Mentor & Erika Frydenlund & Res. Asst. Prof.&VMASC & Agent-based Modeling, Refugees, Forced Migration\\ \midrule
    \multirow{1}{*}{Mentor} & Faryaneh Poursardar & Lecturer & CS & HCI, Digital Libraries, IR, Data Mining\\ \midrule
    \multirow{1}{*}{Mentor} & \multirow{1}{*}{Anne  Perrotti} & \multirow{1}{*}{Asso. Prof.} & \multirow{1}{*}{Education} & Eye Tracking, Adult Learning\\ 
    \bottomrule
    \end{tabular}
\end{table}

%%%%%%%%%%%%%%%%%%%%%%%%%%%%%%%%%%%%%%%%%%%%%%%%%%%%%%%%%%%%
